# Supplementary material for: Monte Carlo Variational Auto-Encoders
Source: arXiv:2106.15921 source file (2021-06-30)
Supplement: Supplementary file 1 [file supplementary.tex]

\section{Proofs}
\label{spsec:proofs}

In the case provided by \Cref{subsec:conditioned_stochastic_flows},  
we can recognize the expression of the weights, writing almost surely,
\[\prod_{k=1}^K w_{u,k}(z_{k-1}, z_{k})  = \frac{\unnormdistr_{K+1}(z_K)}{\unnormdistr_0(z_0)}\Jac_{\Circ{t=1}{K}\propmap{t, u_t}}(z_{0}) \]
which is just the importance weight of the pushforward.
However, we can use this formula to compute an AIS estimator easily with stochastic flows, and in particular write the algorithm for a differentiable AIS with stochastic flow proposals.
\begin{algorithm}[!ht]
    \caption{Differentiable Sequential Sampling with stochastic flow proposals}
    \label{alg:differentiable_ais_flows}
    \begin{algorithmic}
      \STATE {\bfseries Input:}  Number of steps $K$, proposal mappings $\{\propmap{t, u}\}_{t\leq K, u\in\msu}$,  initial distribution $m$, target distribution $\unnormdistr$, annealing schedule $\{\beta_t\}_{t=0}^{K+1}$.
        \\\hrulefill
        \STATE Draw $z_0\sim m$;
        \STATE Set $S_{\Jac} = 0$;
      \FOR{$t=1$ {\bfseries to} $K$}
      \STATE Draw $u_t\sim h_t$;
      \STATE Set $S_{\Jac} = S_{\Jac} + \log \Jac_{\propmap{t, u_t}}(z_{t-1})$;
      \STATE Set $z_t = \propmap{t, u_t}(z_{t-1})$;
\ENDFOR
      \STATE Return $\log \unnormdistr(z_K) - \log m(z_0) + S_{\Jac}$
    \end{algorithmic}
  \end{algorithm}

\subsection{Practical examples of Markov kernels with density of the form \eqref{eq:def_M}}

We give here examples of practical examples of Markov kernels with density that can be written as the marginalisation of a deterministic pushforward $\propmap{u}$, for $u\in\msu$.

Write, for any $x\in\rset^d$, $u\in\msu$, $\propmap{u}(x) = G_x(u)$. Assume that for any $x\in\rset^d$, $G_x$ is a $\rmc^1$-diffeomorphism.
Then, we can write for any positive measurable function $f$,
\begin{align}
    \int M(x, \rmd y) f(y) &= \int f(\propmap{u}(x))\densinnovation(u)\rmd u
    = \int f(G_x(u))\densinnovation(u)\rmd u\\
    &= \int f(v) \densinnovation(G_x^{-1}(v))\Jac_{G_x^{-1}}(v) \rmd v
\end{align}
and the kernel $M$ has a density given by $m(x,y) = \densinnovation(G_x^{-1}(y))\Jac_{G_x^{-1}}(y)$.

In particular, we can exhibit the function, for ULA, 
\begin{equation}
    G_{x}\colon u\mapsto x + \stepsize \nabla \log\pi(x) + \sqrt{2\stepsize} u\eqsp,
\end{equation}
with inverse given by 
\begin{equation}
    G_{x}^{-1}(y) = \{y-x-\stepsize \nabla \log \pi (x)\}/\sqrt{2 \stepsize}\eqsp.
\end{equation}

\section{ELBO AIS}
\label{spsec:ais_elbo}
\subsection{Optimization of the models with the reparameterization trick}

\subsubsection{AIS VAE}
Indeed, we can write the gradient \wrt~$\theta$
\begin{align}
&\nabla_\theta\elboais =  \int \sum_{\chunk{a}{1}{K}}  q_\phi(z_0\mid x) \prod_{t=1}^K \alpha^{a_t}_{t,u_t} \bigl( \Circ{i=1}{t-1} \propmap{i, u_i}^{a_i} (z_0)\bigr)  \densinnovation(u_t) \sum_{t=1}^{K} \nabla_\theta\log  w_t(\Circ{i=1}{t-1} \propmap{i, u_i}^{a_i} (z_0)) \rmd z_0 \rmd \chunk{u}{1}{K}\eqsp,\\
&\widehat{\nabla_\theta\elboais} =\sum_{t=1}^{K} \nabla_\theta\log  w_t(z_{t-1}) = \sum_{t=1}^{K} (\beta_{t}-\beta_{t-1})\nabla_\theta\log p_\theta(x, z_{t-1}) \eqsp,
\end{align}
where $z_0\sim q_\phi(\cdot\mid x)$, $\chunk{u}{1}{K}\sim h$, and recursively for $1\leq t\leq K$,  $a_t\sim\Ber\left(\alpha_{t,u_t} \bigl( z_{t-1}\bigr)\right)$, $z_t = \propmap{t, u_t}^{a_t}(z_{t-1})$.

Moreover, we can differentiate as well with respect to $\phi$, the parameters of the initial distribution and of the proposal mappings of the MH kernels. We rely on the reparameterization trick\arno{rely here again on the trick, you use it for MH}, crucial in optimizing VAEs. Suppose we have access to some diffeomorphism $V_{\phi,x}$ (typically an affine transform, \ie~$V_{\phi,x} (\epsilon)= \mu_\phi(x) + \sigma_\phi(x) *\epsilon$), and some density $\densgauss$ on $\rset^d$,  such that if $\epsilon\sim\densgauss$, then $z_0 = V_{\phi,x}(\epsilon) \sim q_\phi(\cdot\mid x)$. Then we can write
\begin{align}
\nabla_\phi\elboais =&  \int \sum_{\chunk{a}{1}{K}}  \densgauss(\epsilon) \prod_{t=1}^K \alpha^{a_t}_{t,u_t} \bigl( \Circ{i=1}{t-1} \propmap{i, u_i}^{a_i} (V_{\phi,x}(\epsilon))\bigr)  \densinnovation(u_t) \left[\sum_{t=1}^{K} \nabla_\phi\log  w_t(\Circ{i=1}{t-1} \propmap{i, u_i}^{a_i} (V_{\phi,x}(\epsilon)))\right. \\
&+ \left. \prod_{t=1}^{K}  w_t(\Circ{i=1}{t-1} \propmap{i, u_i}^{a_i} (V_{\phi,x}(\epsilon))) \sum_{t=1}^K \nabla_\phi\log\alpha^{a_t}_{t,u_t} \bigl( \Circ{i=1}{t-1} \propmap{i, u_i}^{a_i} (V_{\phi,x}(\epsilon))\bigr)\right]\rmd \epsilon \rmd \chunk{u}{1}{K}\eqsp,\\
\widehat{\nabla_\phi\elboais} &= \sum_{t=0}^{K-1}(\beta_{t+1}- \beta_t)\left[\partial_z\log p_\theta(x,z)\vert_{z= z_t} \partial_\phi  \Circ{i=1}{t} \propmap{i, u_i}^{a_i} (V_{\phi,x}(\epsilon))-\partial_z\log  q_\phi(z\mid x)\vert_{z= z_t}\partial_\phi  \Circ{i=1}{t} \propmap{i, u_i}^{a_i} (V_{\phi,x}(\epsilon)) - \partial_\phi \log  q_\phi(z\mid x)\vert_{z= z_t}\right]  \\
+&\prod_{t=1}^{K}  w_t(z_t)\sum_{t=1}^K \partial_z\log\alpha^{a_t}_{t,u_t} \bigl( z)\bigr)\vert_{z=z_{t-1}} \partial_\phi \Circ{i=1}{t-1} \propmap{i, u_i}^{a_i} (V_{\phi,x}(\epsilon))\eqsp,
\end{align}
where $\epsilon\sim\densgauss$, $\chunk{u}{1}{K}\sim \densinnovation$, $\epsilon\sim\densgauss$ and recursively for $1\leq t\leq K$,  $z_0 = V_{\phi,x}(\epsilon)$, $a_t\sim\Ber\left(\alpha_{t,u_t} \bigl( z_{t-1}\bigr)\right)$, $z_t = \propmap{t, u_t}^{a_t}(z_{t-1})$.
%, and using the remark introduced in \cite{roeder:wu:duvenaud:2017}\arno{could benefit from more details!}.
Note that 
\begin{align}
    \nabla_\phi\log  w_t(\Circ{i=1}{t} \propmap{i, u_i}^{a_i} (V_{\phi,x}(\epsilon))) =& (\beta_{t+1}- \beta_t) \left[\nabla_\phi\log p_\theta(x,\Circ{i=1}{t} \propmap{i, u_i}^{a_i} (V_{\phi,x}(\epsilon))) - \nabla_\phi q_\phi(\Circ{i=1}{t} \propmap{i, u_i}^{a_i} (V_{\phi,x}(\epsilon))\mid x)\right] \\
    =& (\beta_{t+1}- \beta_t)\left[\partial_z\log p_\theta(x,z)\vert_{z= z_t} \partial_\phi  \Circ{i=1}{t} \propmap{i, u_i}^{a_i} (V_{\phi,x}(\epsilon))\right.\\
    &\left.-\partial_z\log  q_\phi(z\mid x)\vert_{z= z_t}\partial_\phi  \Circ{i=1}{t} \propmap{i, u_i}^{a_i} (V_{\phi,x}(\epsilon)) - \partial_\phi \log  q_\phi(z\mid x)\vert_{z= z_t} \right]
\end{align}

\subsubsection{Hierarchical VAE}
In that case, we can obtain again easily an estimator of the gradient \wrt~$\theta$,
\begin{equation}
    \widehat{\nabla_\theta\elbosmc} = \nabla_\theta p_\theta(x, z_K)\,\text{ where }z_0 \sim q_\phi(z_0\mid x)\,,\,\chunk{u}{1}{K}\sim \densinnovation \,,\, z_K=\Circ{t=1}{K}\propmap{t, u_t}(z_{0})\eqsp.
\end{equation}
The estimator of the gradient \wrt~$\phi$ can then itself be written using the reparameterization trick $V_{\phi,x}$
\begin{align}
   \widehat{\nabla_\phi\elbosmc} &= \nabla_\phi \log p_\theta(x, \Circ{t=1}{K}\propmap{t, u_t}(V_{\phi,x}(\epsilon)) - \nabla_\phi\log q_\phi(V_{\phi,x}(\epsilon)\mid x) \\
   &+ \sum_{k=1}^K \nabla_\phi \left[\log l_{k-1}(\Circ{t=1}{k}\propmap{t, u_t}(z_{0}), \Circ{t=1}{k-1}\propmap{t, u_t}(z_{0})) - \log m_k(\Circ{t=1}{k-1}\propmap{t, u_t}(z_{0}), \Circ{t=1}{k}\propmap{t, u_t}(z_{0})) \right]
\end{align}
In particular, if we consider ULA algorithm, or the transitions defined in \cite{huang:tan:lacoste:courville:2018},
write for all $x, u$
\begin{equation}
    \propmap{k,u}(z) = G_{k,z}(u) = \mu_{k,\phi}(z) + \sigma_{k,\phi}(z)*u\eqsp.
\end{equation}
For all $z$, $G_z$ defines a $\rmc^1$ diffeomorphism under mild assumptions.
For ULA, we can directly identify $\mu_\phi(z) = z + \stepsize \nabla_z\log p(x,z)$, $\sigma_\phi(z) = \sqrt{2\stepsize}$, where $\stepsize$ is the stepsize of the ULA transitions.
Finally, we can write $m_k(z_{k-1}, z_k) = \densinnovation(G_{k,z_{k-1}}^{-1}(z_k)) = \densinnovation\left((z_k - \mu_{k,\phi}(z_{k-1})/\sigma_{k,\phi}(z_{k-1}) \right)$, and therefore each of the terms $m_k(\Circ{t=1}{k-1}\propmap{t, u_t}(z_{0}), \Circ{t=1}{k}\propmap{t, u_t}(z_{0})) = \densinnovation(G_{k,\Circ{t=1}{k-1}\propmap{t, u_t}(z_{0})}^{-1}(\Circ{t=1}{k}\propmap{t, u_t}(z_{0})))$ can be optimized.
